# Supplementary material for: VideoRoPE: What Makes for Good Video Rotary Position Embedding?
Source: arXiv:2502.05173 source file (2025-05-30)
Supplement: Supplementary file 1 [file v_niah_d_examples_appendix.tex]

\begin{table*}[h!]
  \begin{center}
  \makebox[\textwidth]{
  \scalebox{1.0}{
    \begin{tabular}{p{4cm} p{10cm}}
      \toprule
      \multicolumn{2}{l}{\bf V-NIAH Needles} \\
      \midrule 
      \\
      \multirow{2}{*}{\includegraphics[width=4cm, height=4cm, keepaspectratio]{figures/files/zoo.png}} & \textbf{Question:} Find the frame of the 'While You Were Out' note. What is the name of the university on that note? \\
      & A. University of California, Los Angeles \\
      & B. University of California, San Diego \\
      & C. University of California, Berkeley \\
      & D. University of California, Santa Barbara \\
      & Answer with the option's letter from the given choices directly.\\
      \\
      & \textbf{Answer:} B \\
      \\
      \\
      \midrule 
      \\
      \multirow{2}{*}{\includegraphics[height=5cm, width=3cm, keepaspectratio]{figures/files/sora_balloon.png}} & \textbf{Question:} Find the frame of a couple in a wedding. Inside the frame, there is a balloon on the bridegroom's head. What is the color of that balloon? \\
      & Answer the question using a single word or phrase. \\
      \\
      & \textbf{Answer:} Yellow \\
      \\
      \\
      \midrule
      \\
      \multirow{2}{*}{\includegraphics[height=5cm, width=3cm, keepaspectratio]{figures/files/selenium_green.jpg}} & \textbf{Question:} Find the frame with the image of Selenium tablets. How many mg does each tablet contain? \\
      & Answer the question using a single word or phrase. \\
      \\
      & \textbf{Answer:} 200 \\
      \\
      \\
      \\
      \midrule 
      \\
      \multirow{2}{*}{\includegraphics[height=5cm, width=3cm, keepaspectratio]{figures/files/panda_scientist.png}} & \textbf{Question:} Find the frame of a scientist. The scientist is a... \\
      & A. Bird \\
      & B. Elephant \\
      & C. Panda \\
      & D. Dog \\
      & Answer with the option's letter from the given choices directly. \\
      \\
      & \textbf{Answer:} C \\
      \\
      \midrule 
      \\
      \multirow{2}{*}{\includegraphics[height=5cm, width=3cm, keepaspectratio]{figures/files/teddy_bear_times_square.png}}  & \textbf{Question:} Find the frame of a teddy bear. Where is this teddy bear? \\
      & A. Times Square \\
      & B. Eiffel Tower \\
      & C. Taj Mahal \\
      & D. Sydney Opera House \\
      & Answer with the option's letter from the given choices directly. \\
      \\
      & \textbf{Answer:} A \\
      \\
      \midrule 
    \end{tabular}
  }
  }
  \end{center}
\caption{The design of the 5 visual question-answering problems used as the needle in V-NIAH.}
\label{tab:vniah-needles}
\end{table*}
