# Supplementary material for: VideoRoPE: What Makes for Good Video Rotary Position Embedding?
Source: arXiv:2502.05173 source file (2025-05-30)
Supplement: Supplementary file 2 [file v_niah_d_periodic_appendix.tex]

% 增加行间距
\setlength{\tabcolsep}{10pt}
\begin{table}[!h]
\centering
\footnotesize
\caption{
Performance comparison of two modeling frequencies, evaluated on V-NIAH-D under identical training conditions. \textit{Random} refers to the average retrieval accuracy when distractors are added randomly. \textit{Periodic} refers to the average retrieval accuracy when distractors are added periodically. 
% High-frequency modeling represents the Baseline (M-RoPE); low-frequency modeling represents the Baseline +  LFTM. 
Each frame is encoded using 144 tokens. A depth interval of 0.2 is used to insert the needle frame. Validation starts with a haystack of 100 frames and progresses at 200-frame intervals, up to 3000 frames. The final result is the average retrieval accuracy across all haystack and depth tests.
}

\label{tab:v-niah-d-periodic-appendix}
\vspace{2mm}
\begin{tabular}{lcc}
\toprule
\textbf{Method} & \textbf{Random} & \textbf{Periodic}  \\ \hline
M-RoPE & 60.89 & 53.11 \\
Ours & \textbf{76.00} & \textbf{68.44} \\
\bottomrule
\end{tabular}
\end{table}
